# Supplementary material for: Monge-Ampere Regularization for Learning Arbitrary Shapes from Point Clouds
Source: arXiv:2410.18477 source file (2025-06-02)
Supplement: Supplementary file 1 [file Supplement.pdf]

# Supplementary Material of "Monge-Ampere Regularization for Learning Arbitrary Shapes from Point Clouds"

Chuanxiang Yang, Yuanfeng Zhou, Guangshun Wei, Long Ma, Junhui Hou, *Senior Member, IEEE*, Yuan Liu and Wenping Wang, *Fellow, IEEE*

## A. Additional Experiments

**Significant Noise.** To evaluate the robustness of our method, we conduct experiments on the MGN dataset [1] with Gaussian noise (standard deviation = 0.003). The baseline approaches include UDF-based approaches: NDF [2], CAP-UDF [3], GIFS [4], GeoUDF [5] and LevelSetUDF [6], as well as SDF-based UDF approaches: NSH [7] and StEik [8]. Quantitative and visual comparisons are provided in Tab. I and Fig. 1, respectively. For results on noise-free data, please refer to Sec. IV-B of the paper. It can be seen that due to its high fidelity to the input point clouds, our method may interpret the noise as surface details when handling point clouds with significant noise, resulting in uneven reconstructed surfaces. To address this issue, we need to reduce the model's fit to the input point clouds with significant noise, as their reliability is not entirely guaranteed. Consequently, we decrease the weights of $L_{Dirichlet}$ and $L_{Neumann}$, which encourage the neural network and its gradient to vanish on the input point clouds, setting the hyper-parameters to ($\lambda_{Dirichlet}$, $\lambda_{Neumann}$, $\lambda_{MA}$, $\lambda_{non-manifold}$) = ($10^7$, $8 \times 10^4$, $8.5 \times 10^{-3}$, $10^6$). As shown in Tab. I and Fig. 1, the results after adjusting the loss weights surpass those of the baseline methods. However, our approach does not currently allow for adaptive adjustment of loss weights based on the noise level, which remains a challenge to be addressed in future work.

TABLE I
QUANTITATIVE COMPARISON OF SURFACE RECONSTRUCTION ON MGN DATASET [1] WITH GAUSSIAN NOISE (STANDARD DEVIATION = 0.003). NOTE THAT THE METHODS MARKED WITH † ARE SUPERVISED, WHICH REQUIRE GROUND-TRUTH DISTANCE VALUES FOR TRAINING. "OURS" AND "OURS*" DENOTE THE RESULTS BEFORE AND AFTER ADJUSTING THE LOSS WEIGHTS, RESPECTIVELY.

| Method | CD ↓ | | Normal ↑ | | F-Score ↑ | |
|---|---|---|---|---|---|---|
| | mean | median | mean | median | mean | median |
| NDF† [2] | 10.286 | 10.394 | 94.59 | 94.82 | 24.82 | 20.91 |
| GIFS† [4] | 5.394 | 5.247 | 86.96 | 87.00 | 83.19 | 85.26 |
| CAP-UDF [3] | 4.619 | 4.556 | 90.85 | 91.62 | 91.76 | 94.40 |
| GeoUDF† [5] | 6.625 | 6.096 | 87.57 | 87.49 | 69.89 | 78.09 |
| LevelsetUDF [6] | 4.336 | 4.125 | 93.99 | 94.08 | 93.86 | **97.12** |
| NSH [7] | 7.775 | 7.999 | 77.55 | 78.92 | 81.90 | 84.75 |
| StEik [8] | 8.731 | 8.640 | 68.18 | 68.31 | 71.23 | 74.41 |
| Ours | 4.240 | 4.364 | 80.41 | 81.16 | 92.70 | 92.86 |
| Ours* | **3.863** | **4.058** | **95.56** | **96.81** | **97.19** | 96.96 |

**Varying Point Density.** We sample 5000, 10000, 20000, 30000, 40000 and 50000 points for each shape from the Stanford 3D Scanning Repository to evaluate the reconstruction quality of our method under different point cloud densities. We visualize how the reconstruction quality of our method varies with different point cloud densities in Fig. 2. Alongside the visual results shown in Fig. 3, we observe that when dealing with sparse point clouds, our method may mistakenly interpret the gaps between neighboring points as intrinsic characteristics of the underlying surfaces due to its high fidelity to the input and ability to represent arbitrary shapes. This leads to holes in the reconstructed surfaces and significant reconstruction errors. The baseline methods are not as sensitive to the gaps between points. This limitation can be addressed by upsampling the point clouds prior to reconstruction, as shown in Figs. 2 and 3.

Chuanxiang Yang, Yuanfeng Zhou, Guangshun Wei, Long Ma are with the School of Software, Shandong University, Jinan 250100, China (e-mail: chxyang2023@gmail.com; yfzhou@sdu.edu.cn; guangshunwei@gmail.com; malong@sdu.edu.cn).

Junhui Hou is with the Department of Computer Science, City University of Hong Kong, Hong Kong (e-mail:jh.hou@cityu.edu.hk).

Yuan Liu is with the College of Computing and Data Science, Nanyang Technological University, Singapore (e-mail: liuyuanwhuer@gmail.com).

Wenping Wang is with the Department of Computer Science and Engineering, Texas A&M University, College Station, TX 77843 USA (e-mail: wenping@tamu.edu).

## REFERENCES

[1] B. L. Bhatnagar, G. Tiwari, C. Theobalt, and G. Pons-Moll, "Multi-garment net: Learning to dress 3d people from images," in *Proceedings of the IEEE/CVF international conference on computer vision*, 2019, pp. 5420–5430.

[2] J. Chibane, G. Pons-Moll *et al.*, "Neural unsigned distance fields for implicit function learning," *Advances in Neural Information Processing Systems*, vol. 33, pp. 21 638–21 652, 2020.

[3] J. Zhou, B. Ma, S. Li, Y.-S. Liu, Y. Fang, and Z. Han, "Cap-udf: Learning unsigned distance functions progressively from raw point clouds with consistency-aware field optimization," *IEEE Transactions on Pattern Analysis and Machine Intelligence*, pp. 1–18, 2024.

[4] J. Ye, Y. Chen, N. Wang, and X. Wang, "Gifs: Neural implicit function for general shape representation," in *Proceedings of the IEEE/CVF Conference on Computer Vision and Pattern Recognition*, 2022, pp. 12 829–12 839.

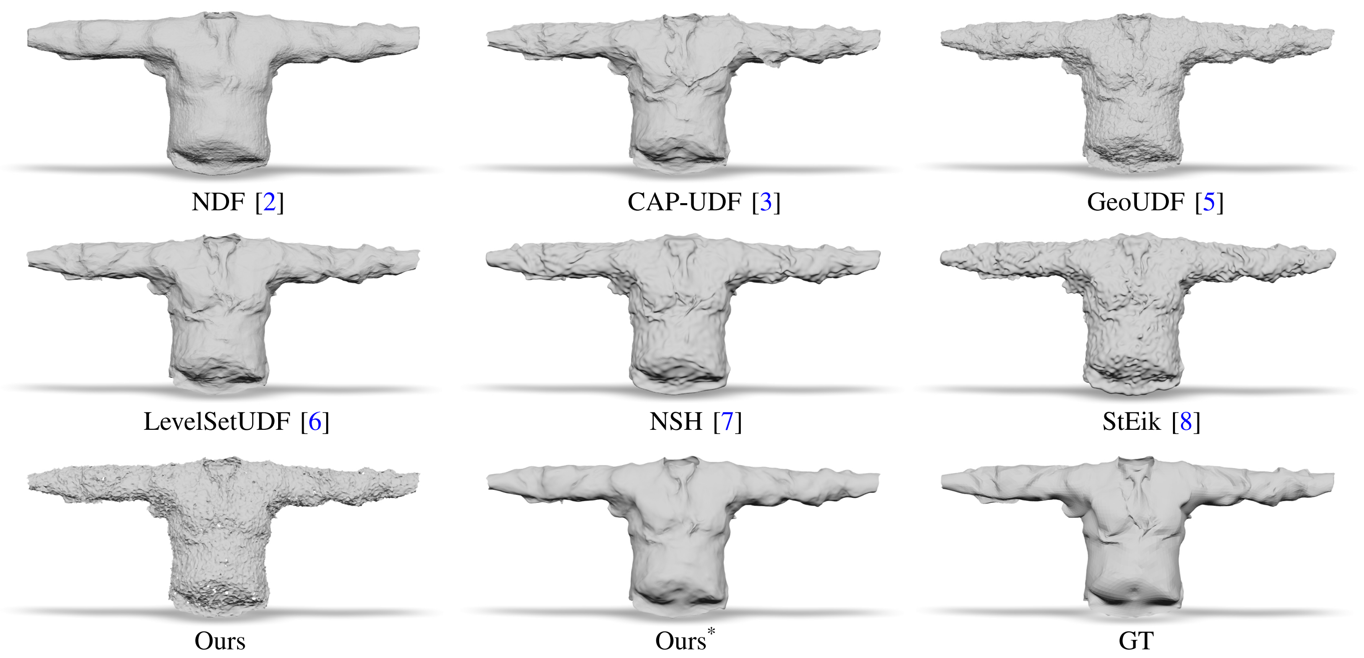


Fig. 1. Visual comparison of surface reconstruction on MGN dataset [1] with Gaussian noise (standard deviation = 0.003). "Ours" and "Ours*" denote the results before and after adjusting the loss weights, respectively.

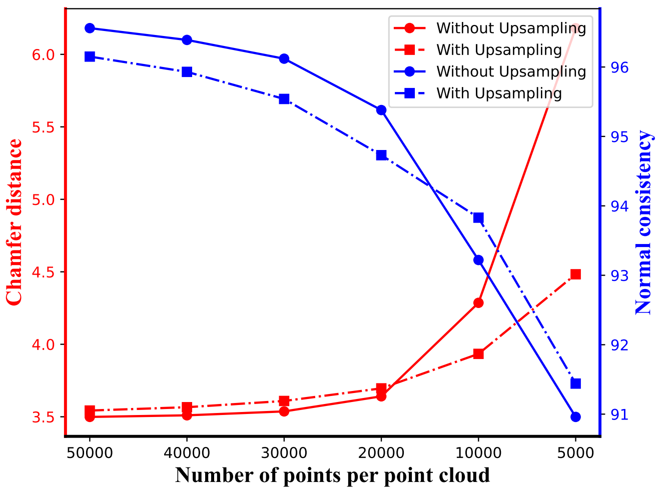


Fig. 2. Variation in reconstruction quality across different point cloud densities on the Stanford 3D Scanning Repository.

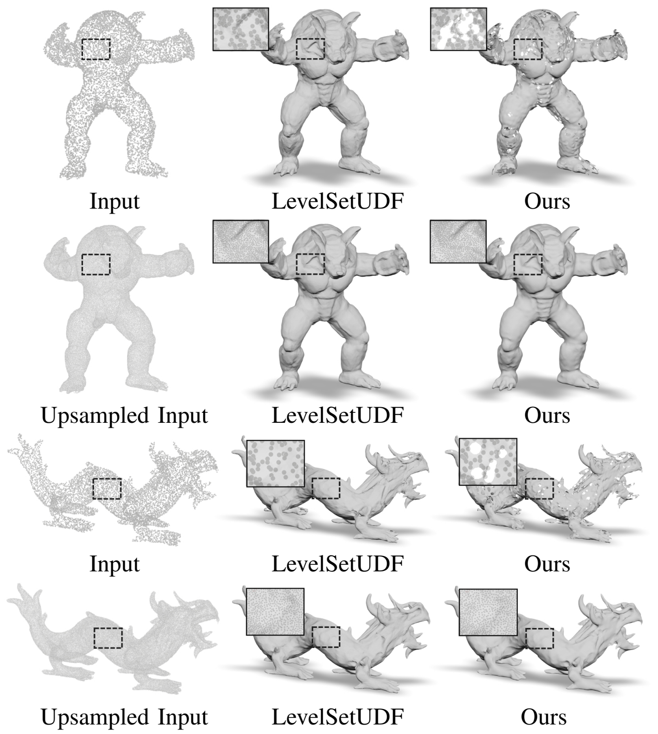


Fig. 3. Visualization of reconstruction results on sparse point clouds. Input contains 10K points.

[5] S. Ren, J. Hou, X. Chen, Y. He, and W. Wang, "Geoudf: Surface reconstruction from 3d point clouds via geometry-guided distance representation," in *Proceedings of the IEEE/CVF International Conference on Computer Vision*, 2023, pp. 14 214–14 224.

[6] J. Zhou, B. Ma, S. Li, Y.-S. Liu, and Z. Han, "Learning a more continuous zero level set in unsigned distance fields through level set projection," in *Proceedings of the IEEE/CVF international conference on computer vision*, 2023, pp. 3181–3192.

[7] Z. Wang, Y. Zhang, R. Xu, F. Zhang, P.-S. Wang, S. Chen, S. Xin, W. Wang, and C. Tu, "Neural-singular-hessian: Implicit neural representation of unoriented point clouds by enforcing singular hessian," *ACM Transactions on Graphics (TOG)*, vol. 42, no. 6, pp. 1–14, 2023.

[8] H. Yang, Y. Sun, G. Sundaramoorthi, and A. Yezzi, "Stabilizing the optimization of neural signed distance functions and finer shape representation," *Advances in Neural Information Processing Systems*, vol. 36, 2024.
